# Supplementary material for: Nonreciprocal amplification toward chaos in a chain of Duffing oscillators
Source: arXiv:2502.01054 ancillary file (2025-06-23)
Supplement: Supplementary file 1 [file zhao2025nonreciprocal_supp.pdf]

**Supplementary Materials for**  
**“Nonreciprocal Amplification toward Chaos**  
**in a Chain of Duffing Oscillators”**

Luekai Zhao, Bojun Li, and Nariya Uchida\*

*Department of Physics, Tohoku University, Sendai 980-8578, Japan*

## SECTION 1: LYAPUNOV FUNCTION

Here, we analytically study the attractors for  $(N,n)=(1,2)$ ,  $C' = C$  using Lyapunov function

$$L(x_1, v_1, x_2, v_2) = \frac{1}{2}(v_1^2 + v_2^2) + \frac{k}{4}(x_1^4 + x_2^4) - \frac{\kappa}{2}(x_1^2 + x_2^2) + \frac{C}{2}(x_1 - x_2)^2 > -\infty. \quad (1)$$

The derivative of  $L(x_1, v_1, x_2, v_2)$  with respect to time is

$$\frac{dL}{dt} = -\gamma(v_1^2 + v_2^2) \leq 0. \quad (2)$$

The derivative of the Lyapunov function is zero within a 2D subspace  $(x_1, 0, x_2, 0)$  and negative otherwise. Since the infimum of  $L(x_1, v_1, x_2, v_2)$  exists, the attractors must reside in the 2D subspace. However, any trajectory cannot stay in the 2D subspace because arbitrary two phase points in the subspace,  $(x_1, 0, x_2, 0)$  and  $(x'_1, 0, x'_2, 0)$ , have no connection when velocity vanishes. Conceptually, the phase points inside the 2D subspace, except three fixed points, are linked to the phase points outside the 2D subspace via the vector field that is perpendicular to the 2D subspace. The flows will converge to the minima as a result of the monotonically decreasing Lyapunov Function. All in all, the fixed points become the only possible attractors in this scenario.

Next, we check the stability of the fixed points. We take the three conspicuous fixed points  $(x_1 = x_2 = 0, v_1 = v_2 = 0)$  and  $(x_1 = x_2 = \pm\sqrt{\kappa/k}, v_1 = v_2 = 0)$  as examples. The purpose is to find whether fixed points are local minima. As  $L(x_1, v_1, x_2, v_2) \geq L(x_1, 0, x_2, 0)$ , it suffices to restrict our analysis to the 2D subspace. The first-order partial derivatives of  $L(x_1, 0, x_2, 0)$  are

$$\partial_{x_1} L = kx_1^3 - \kappa x_1 - C(x_2 - x_1), \quad (3)$$

$$\partial_{x_2} L = kx_2^3 - \kappa x_2 - C(x_1 - x_2). \quad (4)$$

It is obvious that first-order partial derivatives vanish at fixed points. The further validation of local minima requires the computation of the Hessian matrix, which is

$$\begin{pmatrix} \frac{\partial^2 L}{\partial x_1^2} & \frac{\partial^2 L}{\partial x_1 \partial x_2} \\ \frac{\partial^2 L}{\partial x_2 \partial x_1} & \frac{\partial^2 L}{\partial x_2^2} \end{pmatrix} = \begin{pmatrix} 3kx_1^2 - \kappa + C & -C \\ -C & 3kx_2^2 - \kappa + C \end{pmatrix} \quad (5)$$

If the Hessian matrix is evaluated at the fixed points, (5) will be

$$x_1 = x_2 = 0, v_1 = v_2 = 0 : \begin{pmatrix} -\kappa + C & -C \\ -C & -\kappa + C \end{pmatrix}; \quad (6)$$

$$x_1 = x_2 = \pm\sqrt{\kappa/k}, v_1 = v_2 = 0 : \begin{pmatrix} 2\kappa + C & -C \\ -C & 2\kappa + C \end{pmatrix}. \quad (7)$$

The eigenvalues of (6) are  $-\kappa + 2C$  and  $-\kappa$ . Provided that  $-\kappa + 2C < 0$ , (6) is negative definite and  $(x_1 = x_2 = 0, v_1 = v_2 = 0)$  is a local maximum, which represents general cases discussed in the main paper. On the other hand, (7) has 2 positive eigenvalues  $2\kappa$ ,  $2\kappa + 2C$  and is positive definite, making  $(x_1 = x_2 = \pm\sqrt{\kappa/k}, v_1 = v_2 = 0)$  two global minima of Lyapunov function. To conclude, the global minima are attractors whereas local maxima are unstable fixed points.

Although there exist other fixed points, the global minima are always located at  $(x_1 = x_2 = \pm\sqrt{\kappa/k}, v_1 = v_2 = 0)$ . This can be deduced from inequation :

$$L(x_1, v_1, x_2, v_2) \geq \frac{k}{4}(x_1^4 + x_2^4) - \frac{\kappa}{2}(x_1^2 + x_2^2). \quad (8)$$

The global minima of RHS are  $(x_1 = x_2 = \pm\sqrt{\kappa/k}, v_1 = v_2 = 0)$ .

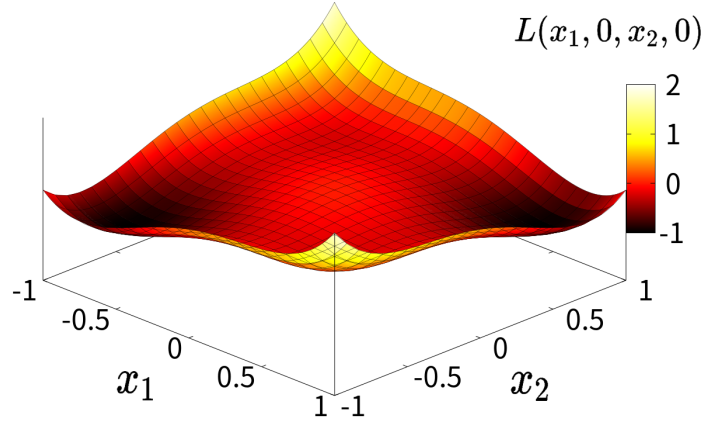

FIG. S1. Lyapunov function in 2D subspace.

FIG. S1 shows the  $L(x_1, 0, x_2, 0)$ . Here,  $k=8$ ,  $\kappa=4$ ,  $C=1$ . As we expect, there are two global minima and one local maximum corresponding to the three fixed points. Such a fact is in accordance with the stability analysis for these three fixed points which gives one unstable fixed point tied to the other two stable fixed points via its unstable manifold. Likewise, the constant negative 1st LLE insists on the existence of fixed points without any bifurcation.

## SECTION 2: THE RECIPROCAL MODEL OF A UNIT

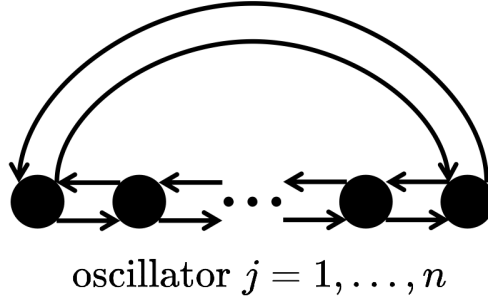

FIG. S2. The reciprocal model of a unit. The solid black circles, black arrows represent dissipative double-well Duffing oscillators and reciprocal couplings  $C$ , respectively.

FIG. S2 provide a conceptual sketch of a contrasting reciprocal model of a unit, which corresponds to the differential equations

$$\dot{x}_j = v_j, \quad \forall j \quad (9)$$

$$\dot{v}_j = \begin{cases} -kx_j^3 + \kappa x_j + C(x_{j-1} - x_j) + C(x_{j+1} - x_j) - \gamma v_j, & j \neq 1 \text{ and } j \neq n \\ -kx_j^3 + \kappa x_j + C(x_n - x_j) + C(x_{j+1} - x_j) - \gamma v_j, & j = 1 \\ -kx_j^3 + \kappa x_j + C(x_{j-1} - x_j) + C(x_1 - x_j) - \gamma v_j, & j = n. \end{cases} \quad (10)$$

Although a ring structure is formed, the indispensable NRSE exemplified by unidirectional couplings is missing now. As the reciprocal system has no amplification effect, the dampening effect cannot be counteracted by the compensation from the ring structure. The resulting attractors are fixed points. To be more specific, a Lyapunov function can be constructed for any reciprocal system according to Section 1. From the analysis in Section 1, the existence of trajectory is excluded from the subspace of zero derivative for the Lyapunov function, making fixed points the only possible attractors.

## SECTION 3: CRITERIA FOR THE FIRST LLE

FIG. S3(a) and FIG. S3(b) justify the interval in which the values of the first LLE are deemed as zero. As we can see, there are evident gaps in both FIG. S3(a) and FIG. S3(b). Therefore, we choose a value within the gap to determine the bound for the interval. The

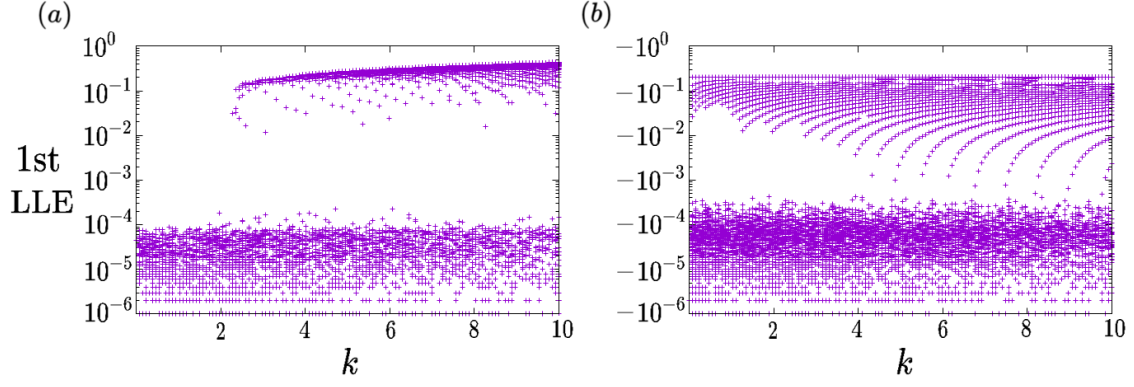

FIG. S3. Projection of 1st LLE to  $k$  axis in  $k$ - $C$  space. (a) Positive value of 1st LLE *vs.*  $k$ . (b) Negative value of 1st LLE *vs.*  $k$ .

resulting interval is  $(-10^{-3}, 10^{-3})$ . As for the value larger than  $10^{-3}$  (smaller than  $-10^{-3}$ ), it is regarded as the positive (negative) first LLE.
